# Supplementary material for: Real-time Hand Tracking under Occlusion from an Egocentric RGB-D Sensor
Source: arXiv:1704.02201 source file (2017-10-05)

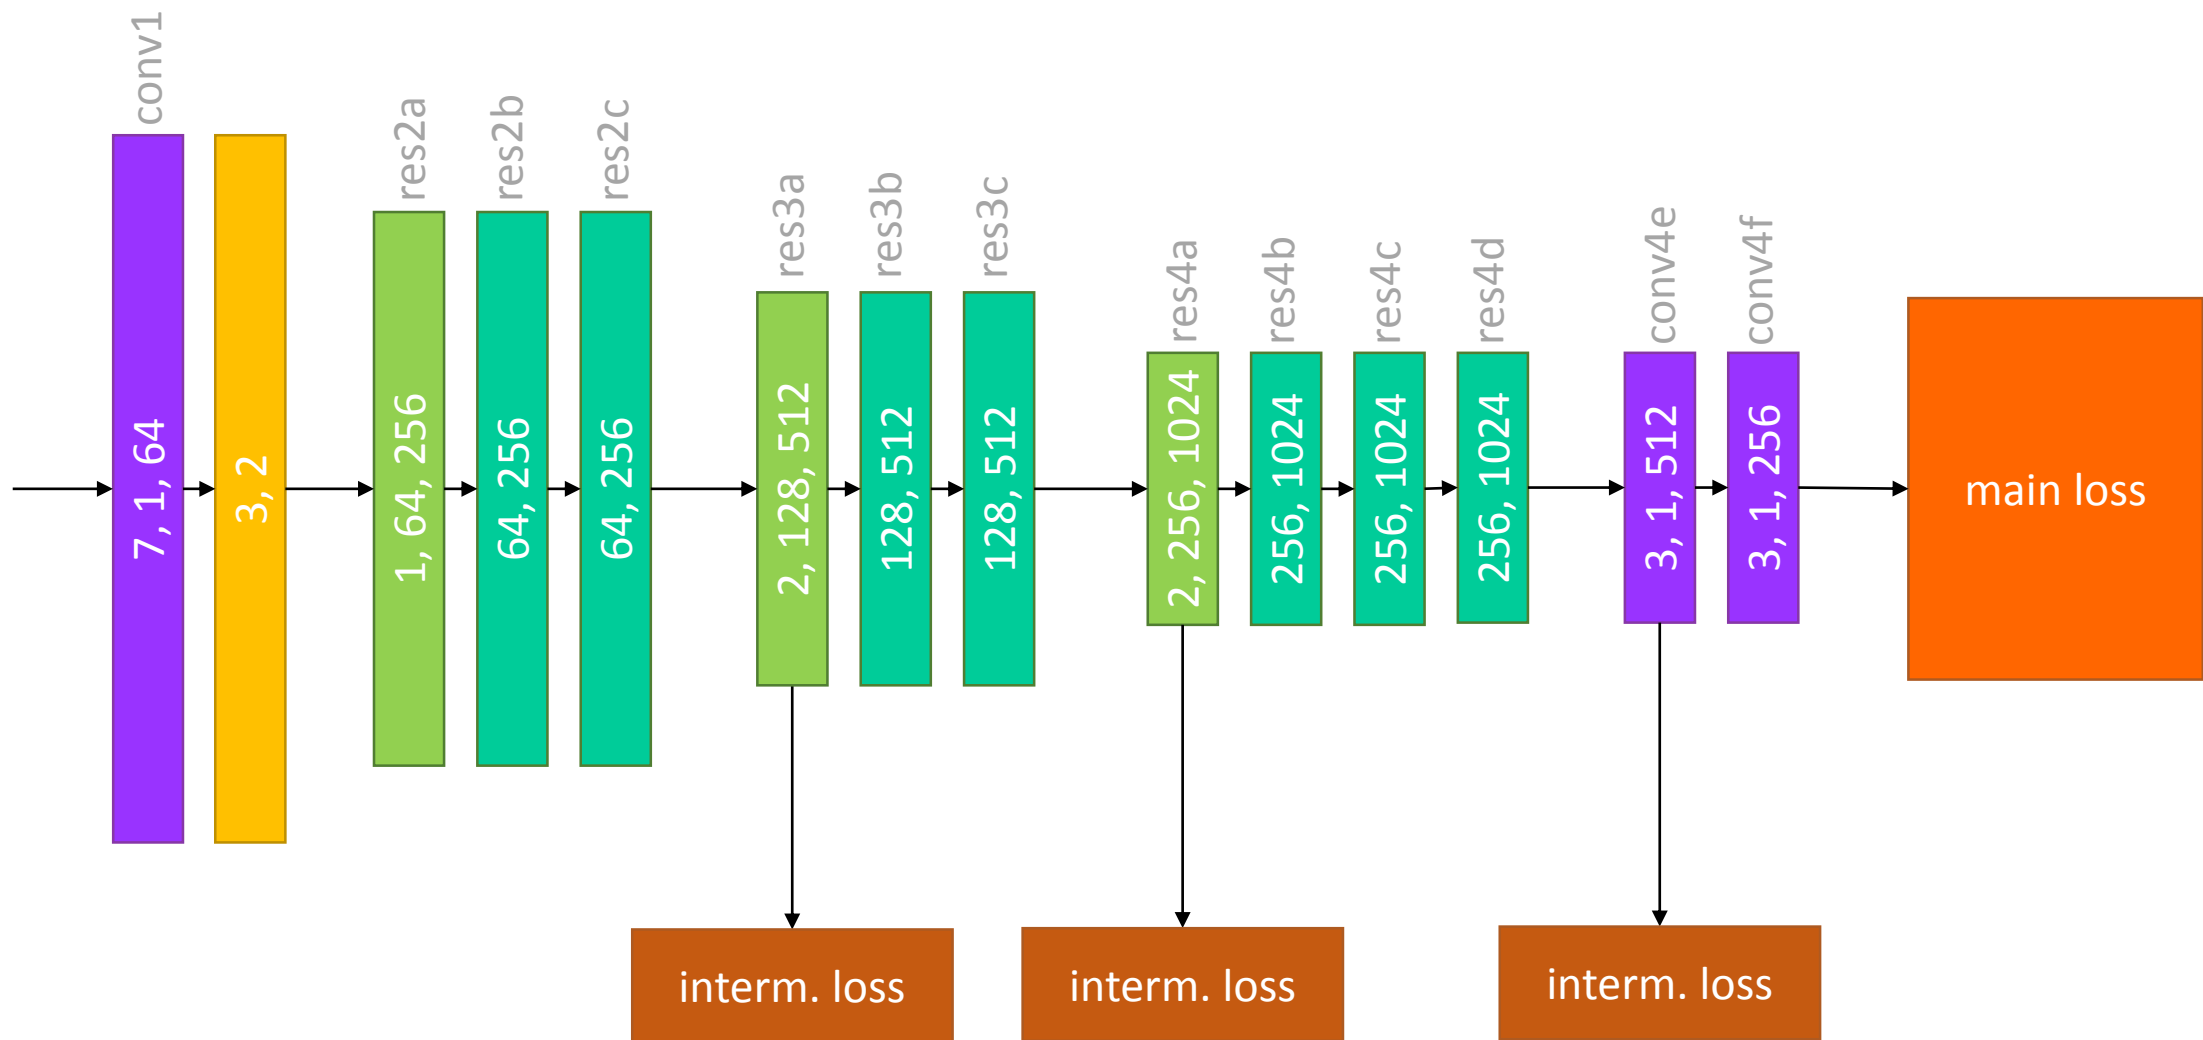

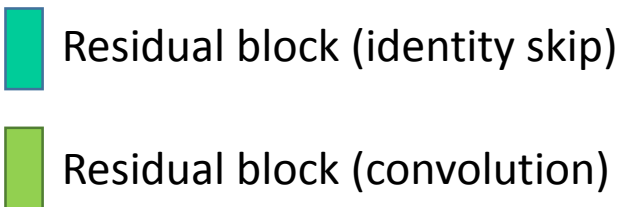 Residual block (identity skip)

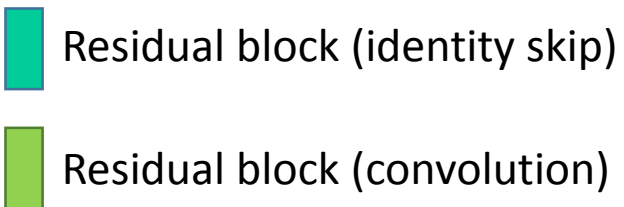 Residual block (convolution)

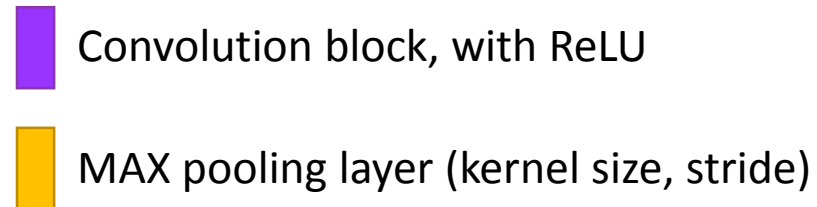 Convolution block, with ReLU

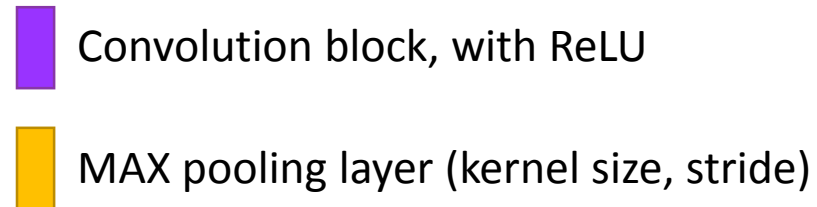 MAX pooling layer (kernel size, stride)

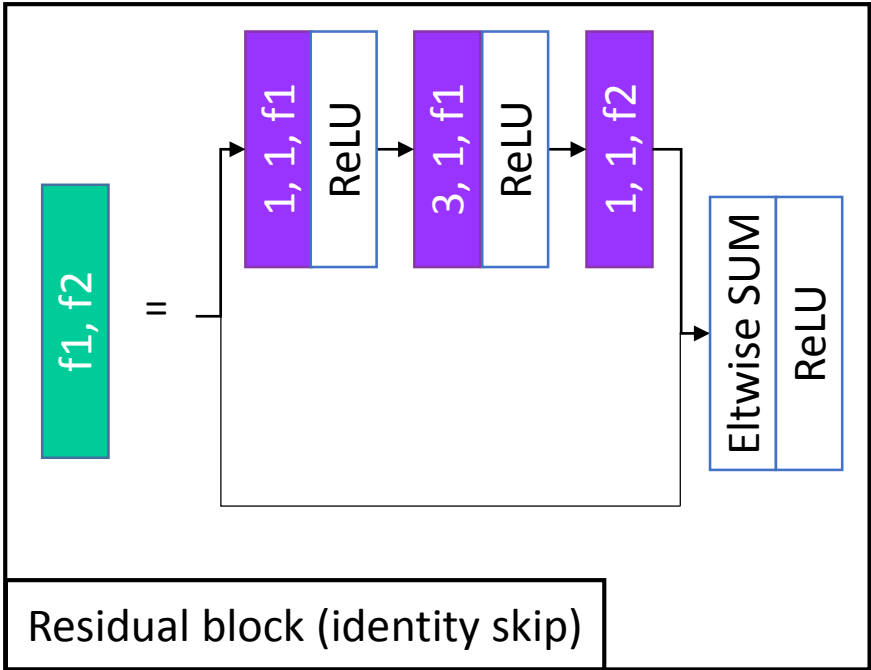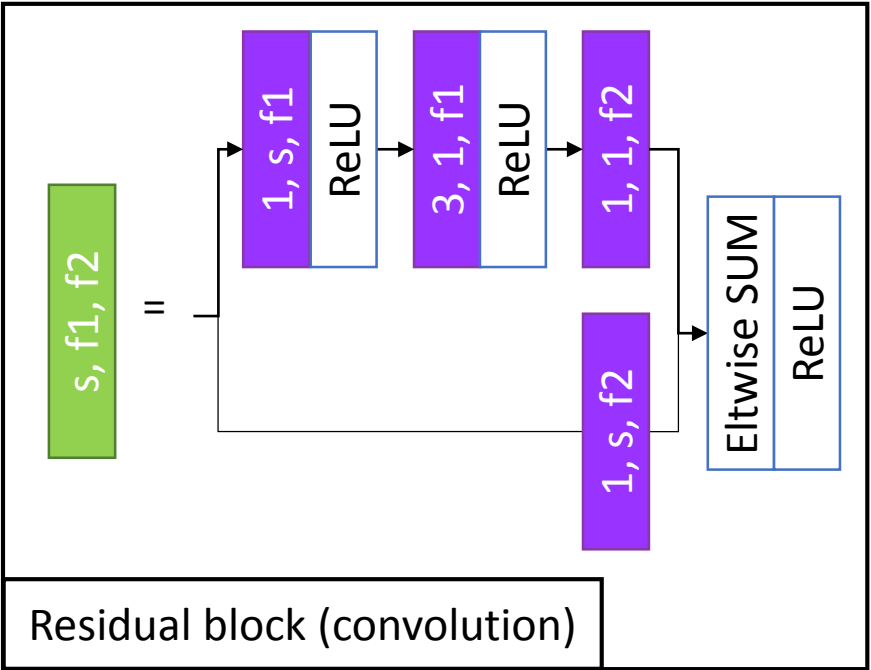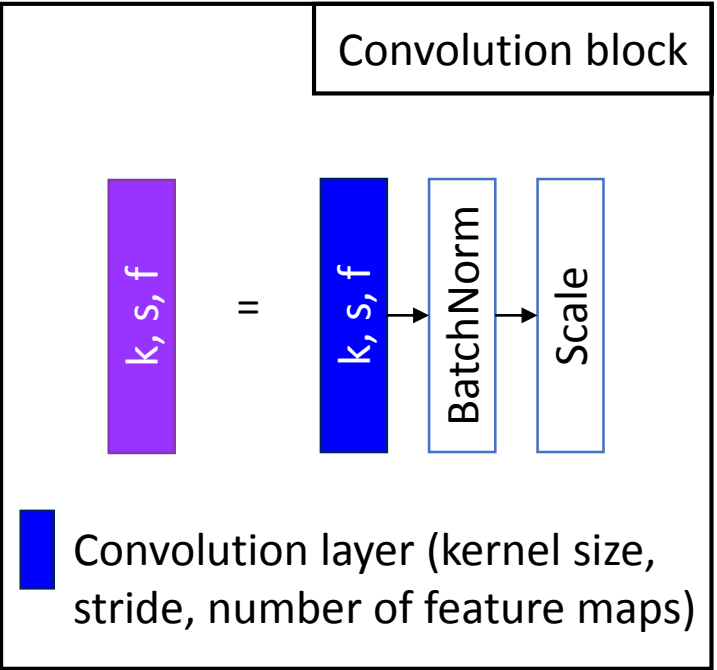

### HALNet / JORNet – Intermediate heatmap loss

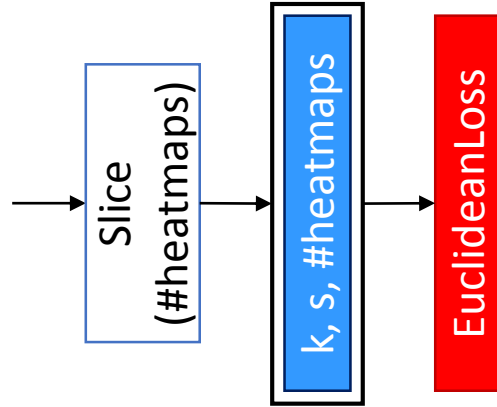

### JORNet – Intermediate joint position loss

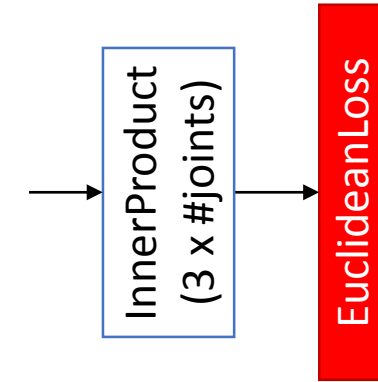

### HALNet – Main loss (heatmaps)

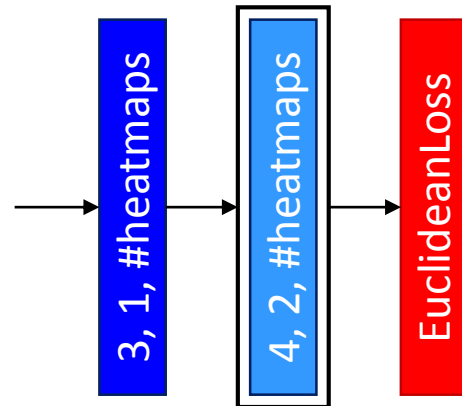

### JORNet – Main loss (joint positions + heatmaps)

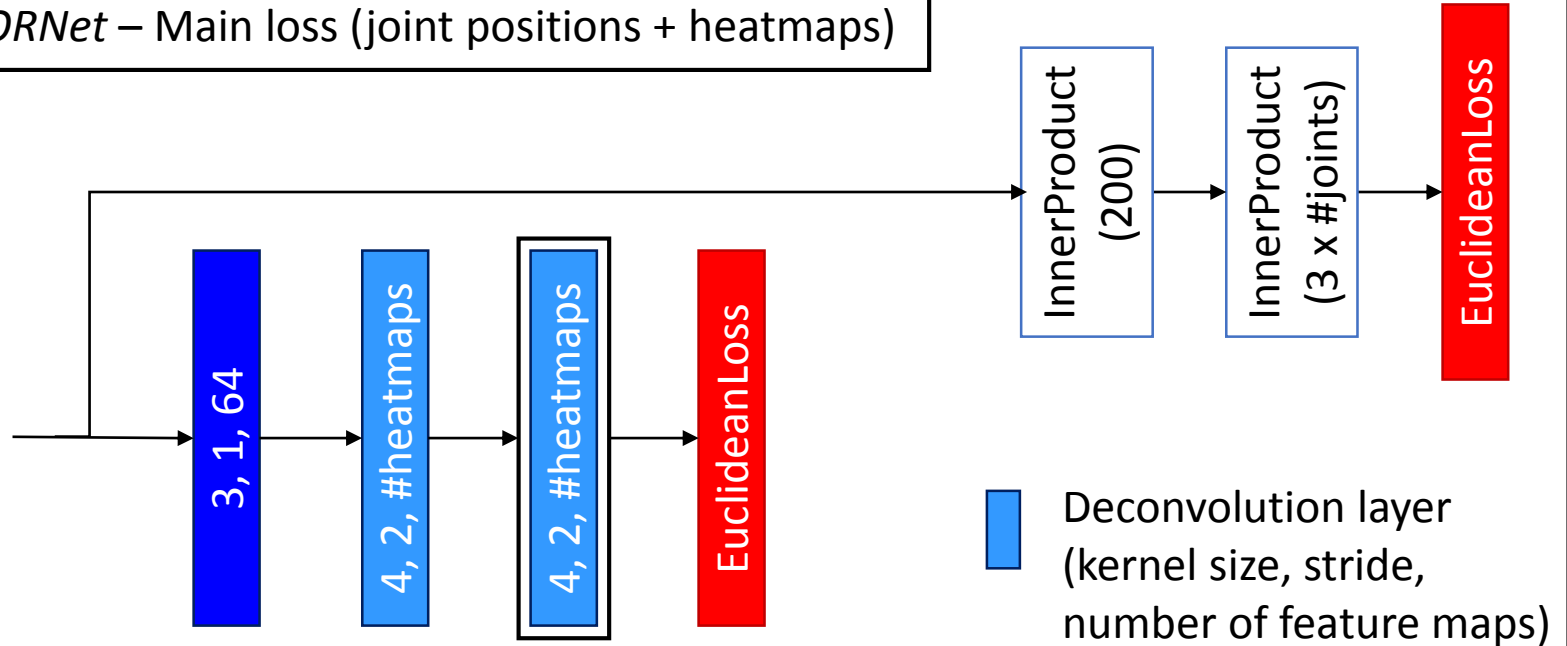

Supplement: Supplementary file 1 [file network.pdf]
